# Supplementary material for: First Observation of Large Missing-Momentum (e,e'p) Cross-Section Scaling and the onset of Correlated-Pair Dominance in Nuclei
Source: arXiv:2209.01492 ancillary file (2022-09-03)
Supplement: Supplementary file 1 [file AoverD_ep_SUPPL.pdf]

# Supplementary Materials

**CLAS detector and particle identification.** The CEBAF Large Acceptance Spectrometer (CLAS) was based on a toroidal magnetic field and had six independent sectors separated by its magnet coils [14]. Each sector included three layers of drift chambers for charged particle momentum and charge determination, and time-of-flight scintillation counters, Cherenkov counters, and electromagnetic calorimeters for particle identification. The in-plane scattering angle coverage of the drift chambers and time-of-flight scintillation counters extended from about $8^\circ$ to $140^\circ$, while that of the Cherenkov counters and electromagnetic calorimeters was more limited, extending from about $8^\circ$ to $45^\circ$. The six sectors collectively covered $50 - 80\%$ of the out-of-plane angle (depending on the in-plane scattering angle).

Electrons were distinguished from pions by their signal in the Cherenkov counters, as well as by a large energy deposition in the electromagnetic calorimeters relative to their momentum. Protons were identified by requiring that their time of flight, measured by the scintillation counters, was consistent to within two standard deviations of the timing measurement resolution, with the calculated time of flight based on the momentum reconstructed in the drift chambers. We applied separate fiducial cuts for electrons and protons to select momentum-dependent regions of CLAS where the detection efficiency was constant and close to 100%.

We used a specialized dual target setup intended to enable precise extractions of $A/d$ cross section ratios [13]. The target consisted of a 2-cm long liquid deuterium target, held inside a thin aluminum cell, followed by an insertable thin solid foil of C, Al, Fe, or Pb. The solid foil was placed 4 cm from the end of the liquid deuterium cell, which allowed us to unambiguously identify which particles originated from the electron interaction with the liquid deuterium and which particles originated from the solid target foil. For each event, the measured electron and proton vertices along the beam direction were required to agree to within 0.8 cm, which corresponds to about two standard deviations of the vertex reconstruction resolution.

**Event Selection for $(e, e'p)$.** We required $Q^2 > 1.5$ (GeV/c)$^2$ and $\theta_{pq} \leq 25^\circ$, i.e., that the knocked-out proton be detected within a $25^\circ$ cone of the momentum transfer vector, $\vec{q}$ [19, 20]. This ensured that the detected proton was the one that absorbed the virtual photon. We also required $350 \leq p_{miss} \leq 600$ MeV/c for the scaling studies, but relaxed that requirement when studying the transition to scaling.

Rather than cutting solely on the missing-mass to select QE contributions and reject inelastic events, we used a loose missing-mass cut and an $x_B$-dependent cut on $\theta_p mq$, the angle between $\vec{p}_{miss}$ and $\vec{q}$. The missing mass was

defined for an electron scattering from a stationary two-nucleon pair:

$$M_{miss}^2 = (\omega + m_d - E_p)^2 - |\vec{q} - \vec{p}_p|^2, \tag{1}$$

where $E_p = \sqrt{|\vec{p}_p|^2 + m^2}$ is the proton energy and $m_d \approx 2m$ is the deuteron mass. In reality, the two-nucleon pair has a binding energy $E^*$ and a non-zero pair center-of-mass (CM) momentum $\vec{p}_{CM}$, which broadened the missing mass distribution.

Fig. S1 shows the measured $M_{miss}$ (see Eq. 1) distribution for $^{12}$C$(e, e'p)$ events for different bins of $x_B$. There is a peak at the nucleon mass due to quasielastic proton knockout and a background at larger missing mass due to inelastic scattering from nucleons resulting in meson production. Since the minimum $p_{miss}$ increases with $x_B$ for $x_B > 1$, at high-$x_B$, where most previous measurements were done, only QE events are seen. We cut on $0.8 \leq M_{miss} \leq 1.08$ GeV/c$^2$ $\approx m + m_\pi$ (where $m_\pi$ is the pion mass), to suppress most inelastic contributions. However, due to broadening, inelastic events extend to lower missing mass and cannot be cleanly separated by a simple cut on $M_{miss}$. Since the functional form of the inelastic background is not known, fitting the background would lead to very large uncertainties.

Therefore we adopted the method of Ref. [4, 26] and used $\theta_{\vec{p}_{miss},\vec{q}}$, the angle between $\vec{p}_{miss}$ and $\vec{q}$, to separate QE and inelastic events (see Fig. S2). In non-QE (inelastic) reactions the momentum transferred to undetected particles shifts the direction of $\vec{p}_{miss}$ and increases $\theta_{\vec{p}_{miss},\vec{q}}$. In contrast to the missing-mass spectra, $\theta_{\vec{p}_{miss},\vec{q}}$ is well described by a two-Gaussian fit. We fit the $\theta_{\vec{p}_{miss},\vec{q}}$ distribution with two Gaussians and selected the cut-off angle between the QE and background events as the point where the two Gaussians intersected. This suppressed the vast majority of the inelastic events while keeping most of the QE events. The contamination due to inelastic events (false positives) was partially balanced by the loss of elastic events (false negatives). In addition, the remaining fractional contribution of the inelastic events in the QE region is similar in both the heavy nuclei and the deuterium spectra and therefore largely cancels in their ratios. As in the $M_{miss}$ spectra, the inelastic peak decreases rapidly as $x_B$ increases above 1.1.

The effect of the $\theta_{\vec{p}_{miss},\vec{q}}$ cut on the missing mass distribution is shown in Fig. S1 where the dashed histograms show the missing-mass distributions separately for events above and below the cut. This cut thus identifies the inelastic tail that extends into the QE region. The small-$\theta_{\vec{p}_{miss},\vec{q}}$ events in the $M_{miss}$ distribution are well described by a Gaussian. This is an encouraging observation that shows that our procedure results in similar performance to those of the traditional peak+background fit procedure, but using well defined kinematical cuts that are suitable for QE scattering studies, and allow for direct comparison with theoretical calculations.

We varied the $\theta_{\vec{p}_{miss},\vec{q}}$ cut to show that our results are not sensitive to the specific method of removing the inelastic contributions (see Fig. S4). Varying the angular cut by $\pm 5^{\circ}$ and even removing it entirely did not significantly change the cross section ratios. This shows that the effect of the residual inelastic contributions largely cancels in the cross section ratio.

The systematic uncertainties associated with our event selection cuts, including the inelastic suppression cuts, are discussed below.

**Cross section extraction.** The reported per-nucleon cross section ratios were extracted from the measured number of $(e, e'p)$ events originating from the solid and liquid deuterium targets by normalizing them by the integrated measured per-nucleon luminosity, and applying corrections for experimental effects such as acceptance and electron radiative effects, as well as for nucleon attenuation effects. The general expression for the per-nucleon $(e, e'p)$ $A/d$ cross section ratio for a given $x_B$ bin is given by:

$$\frac{\sigma_A/A}{\sigma_d/2}(x_B) = \frac{Y^A_{(e,e'p)}(x_B)}{Y^d_{(e,e'p)}(x_B)} \times Acc_{A/d}(x_B) \times RC_{A/d}(x_B) \times \frac{T_d}{T_A}, \tag{2}$$

where $Y^A_{(e,e'p)}(x_B)$ and $Y^d_{(e,e'p)}(x_B)$ are the measured number of $(e, e'p)$ events from target $A$ or $d$, respectively, in a given $x_B$ bin normalized by luminosity, $Acc_{A/d}(x_B)$ is the relative acceptance of the CLAS detector for $(e, e'p)$ events originating from the solid foil target relative to those from the liquid deuterium target, $RC_{A/d}(x_B)$ is the ratio of the nucleus $A$ and $d$ radiative correction factors, and $T_A$ and $T_d$ are transparency factors accounting for the attenuation of nucleons as they exit nucleus $A$ or nucleus $d$.

Deuteron yield. To determine the deuteron event yield, $Y^d_{(e,e'p)}(x_B)$, we separated events originating from interactions with deuterium nuclei and with the aluminum end caps of the target cell. We minimized the end cap contributions by only considering events with an interaction vertex reconstructed to within the central 1 cm of the 2-cm liquid target. We then used measurements with an empty target cell to estimate the remaining cell wall contributions. These contributions were independent of $x_B$ and less than 2% of the measured event yield. We thus reduced the measured yield by 2% and accounted for the uncertainty in this subtraction in our systematic uncertainties.

Acceptance Corrections. We corrected the cross section ratio for the slightly different experimental acceptances for events originating in the 2-cm liquid deuterium target and events originating in the solid target foil located 5-cm downstream from the liquid target center. This factor should be small because the target separation is much smaller than the distances from the targets to the detectors. We estimated this correction factor using a Geant simulation of

CLAS [24]. We generated separate acceptance maps for electrons and for protons originating from a solid target or from the liquid target as a function of particle momentum and in- and out-of-plane scattering angles. We then used the acceptance maps to calculate the acceptance probability for each experimental event as follows. For each event, we rotated the entire event (both electron and proton) by a random angle $\phi$ around the beamline and then rotated the proton momentum by a random angle $\phi'$ around $\vec{q}$. We then used the acceptance maps to determined the probability that the rotated event, which has approximately the same cross section as the measured event, would have been detected by CLAS. We did this calculation separately for events from the liquid and solid targets, accounting for the target position when constructing the acceptance maps. This procedure was repeated 100 times for each event. The acceptance weight for that event equalled 100 divided by the total probability that each of those 100 rotated events would have been detected. The average acceptance weight as a function of $x_B$ for each target is shown in Fig. S5 (left panel). We then took the ratios between the solid- and liquid target acceptance weights to determine $Acc_{A/d}(x_B)$, the cross section ratio acceptance-correction factor for each $x_B$-bin (see Fig. S5, right panel). The uncertainties in $Acc_{A/d}(x_B)$ were added in quadrature to the point-to-point statistical uncertainties of the data.

Radiative and Coulomb effects. The radiative correction factors were determined by calculating the ratio between the Born cross section and the cross section including electron-radiative effects. The latter uses the peaking approximation [28] as implemented in Ref. [22]. The cross sections for the solid targets were calculated using the GCF model and the deuteron cross sections were calculated with the AV18 momentum distribution, as described below. As part of the modified electron kinematics, we also used the Effective Momentum Approximation [29] to account for Coulomb effects that accelerate the incoming electron and knockout proton and decelerate the scattered electron by an energy $\Delta E$, see Ref. [22] for details. We used $\Delta E$ values of 0, 2.9, 5.6, 9.4 and 20.3 MeV for $d$, C, Al, Fe and Pb targets, respectively. The resulting radiative correction factors, $RC_{A/d}(x_B)$, are shown in Fig. S6.

Transparency Corrections. After the electron scatters from a proton, the proton needs to travel through the residual nucleus to be detected. If the proton rescatters too much from the other nucleons, then it will fall outside our event acceptance cuts. The probability of the proton to be detectable after exiting from the nucleus depends on the size of the nucleus. The nuclear transparency probabilities were calculated within a Glauber approximation using an effective scattering cross section. The probability that a proton escapes the nucleus without further interaction is given by:

$$T_A = \frac{1}{A}\int d^3r\rho(r)\exp\left[-\sigma_{eff}\int \rho(z)dz\right], \tag{3}$$

where $\rho(r)$ is the nuclear density distribution (assumed symmetrical), $\rho(z)$ is the nuclear density along the path of the

exiting proton, and $\sigma_{eff}$ is the effective nucleon-nucleon cross section. For the $1-3$ GeV/c protons in this analysis, $\sigma_{eff} = 37 \pm 7$ mb. This gives nuclear transparencies $T_A$ of $1, 0.53 \pm 0.05, 0.43 \pm 0.05, 0.34 \pm 0.04$ and $0.22 \pm 0.03$ for $d$, C, Al, Fe and Pb, respectively.

**Theoretical cross section calculations.** The $(e, e'p)$ nucleon-knockout cross section for high-$Q^2$ reactions is modeled here using a factorized plane wave impulse approximation (PWIA) [30]:

$$\frac{d\sigma_{A(e,e'p)}}{d\Omega_{k'} dE_{k'} d\Omega_p dE_p} = p_p E_p \sigma_{ep} S^N_A(p_{miss}, E_{miss}), \tag{4}$$

where $(\vec{k}', E_{k'})$ is the scattered electron four-momentum, $\sigma_{ep}$ is the off-shell electron-nucleon cross section, and $S^N_A(p_{miss}, E_{miss})$ is the nuclear spectral function for nucleus $A$, which defines the probability for finding a nucleon in the nucleus with momentum $p_{miss}$ and energy $E_{miss}$ (in the following for brevity we drop the "miss" subscript):

$$S^N_A(\mathbf{p}, E) = \sum_n |\langle \Psi^A_0 | [|p\rangle \, |\Psi^{A-1}_n\rangle]|^2 \qquad \times \delta(E + E^A_0 - E^{A-1}_n)\,.$$

where $|p\rangle$ is the single-nucleon state, $|\Psi^A_0\rangle$ is the ground state of the Hamiltonian with energy $E_0$, whereas $|\Psi^{A-1}_n\rangle$ and $E^{A-1}_n$ are the energy eigenstates and eigenvalues of the $(A-1)$-nucleon system. Note that the single-nucleon momentum distribution is recovered by integrating the spectral function over the removal energy $n^N_A(\mathbf{p}) = \int dE S^N_A(\mathbf{p}, E)\,.$

From the above relations, it is clear the deuterium spectral function equals the momentum distribution times a delta function in missing energy. To construct it, we used the AV18 deuterium momentum distribution from Ref. [31].

For nuclei with $A > 2$, we considered two models for spectral function, for the mean-field and for the SRC region. The mean-field component $S^{MF}_N(\mathbf{p}, E)$ corresponds to restricting the sum of Eq. 5 to the bound $A-1$ states

$$S^{N,\,MF}_A(\mathbf{p}, E) = \sum_n |\langle \Psi^A_0 | [|p\rangle \otimes |\Psi^{A-1}_n\rangle]|^2 \qquad \times \delta\Big(E - B^A_0 + B^{A-1}_n - \frac{\mathbf{p}^2}{2m^{A-1}_n}\Big)\,,$$

where $B^A_0$ and $B^{A-1}_n$ are the binding energies of the initial and the $A-1$ remnant nucleus left in a state $n$ with mass $m^{A-1}_n$. The p-shell momentum-space overlaps $\langle \Psi^A_0 | [|p\rangle \otimes |\Psi^{A-1}_n\rangle$ are computed by Fourier transforming the Quantum Monte-Carlo (QMC) radial overlaps for the transitions [32]:

$$^{12}\mathrm{C}(0^+) \to^{11} \mathrm{B}(3/2^-) + p^{12}\mathrm{C}(0^+) \to^{11} \mathrm{B}(1/2^-) + p^{12}\mathrm{C}(0^+) \to^{11} \mathrm{B}(3/2^-)^* + p\,.$$

The quenching of the spectroscopic factors (i.e. the de-occupancy of shell model orbitals due to many body correlations) automatically emerges from the QMC calculations, as they encompass multi-nucleon correlations generated by the highly-realistic AV18 + UX Hamiltonian [33]. This calculation is not available for heavier nuclei.

Computing the $s$-shell mean-field contribution would in principle require evaluating the spectroscopic overlaps for the transitions $^{12}\mathrm{C}(0^+) \rightarrow ^{11}\mathrm{B}(1/2^+)^* + p$ for all the possible excited states of $^{11}$B with $J^P = (1/2^+)$. This procedure involves non-trivial difficulties for the QMC method, which is best suited to study ground-state properties. To circumvent them, we model the $s$-wave single-particle orbitals using harmonic oscillator and Woods-Saxon one-body potentials. We adjust the value of the oscillator frequency $\hbar\omega$ and the parameters of the Wood-Saxon potential so that the Fourier transform of the (quenched) $p$-wave orbitals reproduce that of the QMC. The quenching factor of the $s$-wave orbital is fixed to reproduce the integrated strength of the QMC momentum distribution up to $k_F$. As an alternative strategy, we also calculated the QMC overlap associated with the $^4\mathrm{He}(0^+) \rightarrow ^3\mathrm{H}(1/2^+) + p$ transition. Since nuclear correlation effects are already included in this QMC overlap, only minimal changes to the quenching factor are needed to reproduce the integral of the momentum distribution up to $k_F$. As shown in Fig. S7, the QMC total momentum distribution agrees well with the ones computed by adding the QMC $p$-wave overlap and the $s$-shell overlap obtained from the harmonic oscillator (HO), Wood Saxon (WS) and $^4\mathrm{He}(0^+) \rightarrow ^3\mathrm{H}(1/2^+) + p$ calculations.

We constructed the spectral-function energy dependence using the experimental values for the binding energies of the ground state of $^{12}$C and for the states $^{11}\mathrm{B}(3/2^-)$, $^{11}\mathrm{B}(1/2^-)$, and $^{11}\mathrm{B}(3/2^-)^*$. The energy conserving $\delta$-function of Eq. 5 is parametrized using a narrow Gaussian distribution whose widths are fixed so as to reproduce the missing energy spectra of the $(e, e'p)$ data of Ref. [34]. This data set has also been used to determine the energy centroid and width for the $^{12}\mathrm{C}(0^+) \rightarrow ^{11}\mathrm{B}(1/2^+)^* + p$ $s$-shell transition. Note that the mean-field spectral function already accounts for the reduced occupancy of mean-field states due to multi-nucleon correlations, as the normalization of the spectroscopic overlaps is fixed by QMC calculations. Since the integral is fixed, changing the width of the Gaussian distributions changes the peak heights in the missing-energy spectral function. We varied the widths by 10% to determine the dependence of the results on the widths. We used the cross section variation due to using the different $s$-shell calculations as an uncertainty for the QMC calculations in Fig. 3.

The SRC spectral functions for C, Al, Fe and Pb were modeled using the GCF model [8, 12, 21] following the implementation of Ref. [22] with the AV18 two-nucleon interaction, using pair CM motion width of $150 \pm 20$ MeV/c, and an $A - 2$ excitation energy of $0 - 30$ MeV. The contacts (the probability of finding an SRC pair) were taken from [8].

The complete deuterium spectral function was calculated exactly using the AV18 nucleon-nucleon interaction [31].

The calculated cross sections were integrated over the CLAS experimental acceptance, using the same event selection

cuts as the data, and smeared to account for the CLAS experimental resolution.

**Systematic Uncertainties.** There were several sources of systematic uncertainties, including both point-to-point and correlated uncertainties.

Coulomb Correction: There is a 10% uncertainty in the Coulomb potential ($\Delta E$) used for the Coulomb correction described above. Varying $\Delta E$ by $\pm 10\%$ changed the extracted cross section ratios by a maximum of 3% (for lead). We conservatively chose to use 3% as the point-to-point systematic uncertainty due to Coulomb correction for all targets and all bins.

Event Selection: We varied each of the event selection cuts within reasonable limits (see Table S1) to see the effect of these cuts on the resulting cross section ratios. We repeated the analysis 100 times, choosing the value of each selection cut randomly from a Gaussian distribution centered at the nominal value with a width reflecting a reasonable variation of the cut. We used the mean and variance in the resulting distribution of 100 cross section ratios to define the value of cross section ratio and its event selection cut uncertainty, respectively. These bin-dependent (point-to-point) uncertainties ranged from 4.5% to 12.5%.

Inelastic Background Rejection: We varied the $\theta_p mq$ cut by $\pm 5^\circ$ to see the effect of the differential inelastic background on the cross section ratios (see Fig. S4). We added a point-to-point systematic uncertainty equal to the cross section ratio difference between the $+5^\circ$ and $-5^\circ$ cuts divided by $\sqrt{12}$.

Transparency: The largest normalization systematic uncertainty is due to the transparency correction. It is driven by the uncertainties in the effective nucleon scattering cross sections used for the Glauber calculations that result in 10% (for carbon) to 15% (for lead) uncertainties in the ratios of transparencies of the solid target nuclei to deuterium, see Ref. [19].

Combining different deuteron run periods: We measured electron scattering from deuterium and from each solid target simultaneously. In order to increase the deuterium statistics, we combined the deuterium data from all of the solid target runs. This reduced the statistical uncertainty of the cross section ratios but introduced a systematic uncertainty due to the stability of the beam charge measurement that does not fully cancel in the $A/d$ cross section ratio. This uncertainty was estimated as half of the difference between the total averaged and the individual deuteron normalized yields. The maximum difference was 1.5%, which we used as a normalization systematic uncertainty.

**Inclusive Scaling Measurements.** Previous scaling studies identified scattering from high-momentum nucleons by

measuring the inclusive $(e, e')$ reactions at large $Q^2$ and $x_B$. For a given $x_B$ and $Q^2$, there is a minimum nucleon momentum for absorbing the virtual photon. This minimum momentum increases with $x_B$. It also depends on whether the missing momentum is carried by one other nucleon (for scattering from the deuteron or from a nucleon in an SRC pair) or by the other $A-1$ nucleons of the residual nucleus (for scattering from a mean-field nucleon) [16].

For $Q^2 \geq 1.5$ GeV/c$^2$, the cross section ratio of nuclei to deuterium is independent of $x_B$ for $1.5 \leq x_B \leq 1.9$ [6, 9, 16–18], a phenomena we call scaling. The value of the cross section ratio in the scaling region is interpreted as a measure of the relative number of nucleons in SRC pairs in the measured nuclei. These inclusive studies also determined the onset of scaling to be $275 \pm 25$ MeV/c [6] from $x_B = 1.5 \pm 0.05$ at $Q^2 = 1.4$ GeV$^2$, where scaling starts. This is somewhat larger than the Carbon Fermi momentum and consistent with our results.

However, recent studies [35] show that the relation between $Q^2$, $x_B$, and the minimal initial nucleon momentum also depends on the detailed characteristics of SRC pairs, such as their center-of-mass (CM) motion and the excitation energy of the residual nuclear system. This prevents a precise determination of the SRC scaling onset from the high-$x_B$ $(e, e')$ scaling measurements.

In contrast, the $(e, e'p)$ reaction used in this paper is insensitive to such model details since detecting the proton allows us to directly determine $\vec{p}_{miss}$ for each event, thereby enabling a complementary and precise determination of the SRC scaling onset.

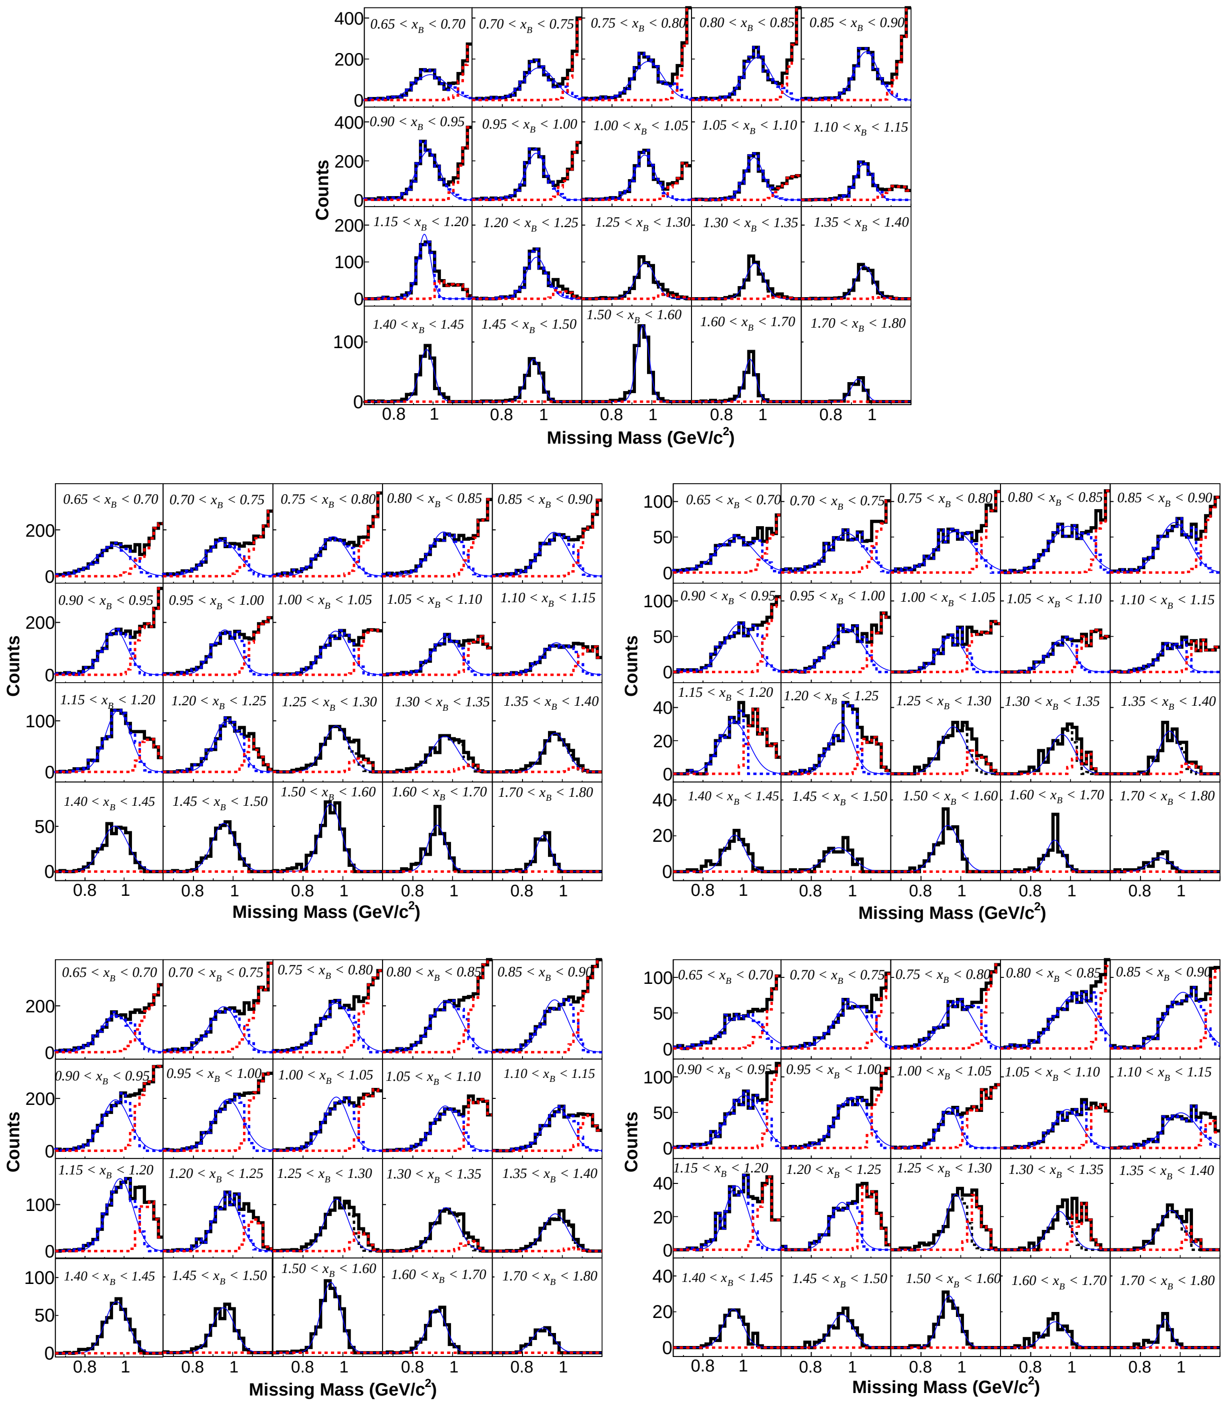


**Fig. S1: Missing Mass distributions.** Number of events plotted vs. $M_{miss}$ for the $(e, e'p)$ reaction for different bins of $x_B$ for D (top), C (middle left), Al (middle right), Fe (bottom left), and Pb (bottom right). The data were cut on $Q^2 \geq 1.5$ GeV$^2$, $\theta_{pq} \leq 25^{\circ}$, and $350 \leq p_{miss} \leq 600$ MeV/c. The black histogram represents all events. The blue dashed histogram shows the data cut on $\theta_{\vec{p}_{miss},\vec{q}}$, the opening angle between the missing momentum $\vec{p}_{miss}$ and the virtual photon $\vec{q}$, as determined in Fig. S2. The red dashed histogram shows the events failing the $\theta_{\vec{p}_{miss},\vec{q}}$ cut. The thin solid blue line shows the Gaussian fit to the blue dashed histogram.

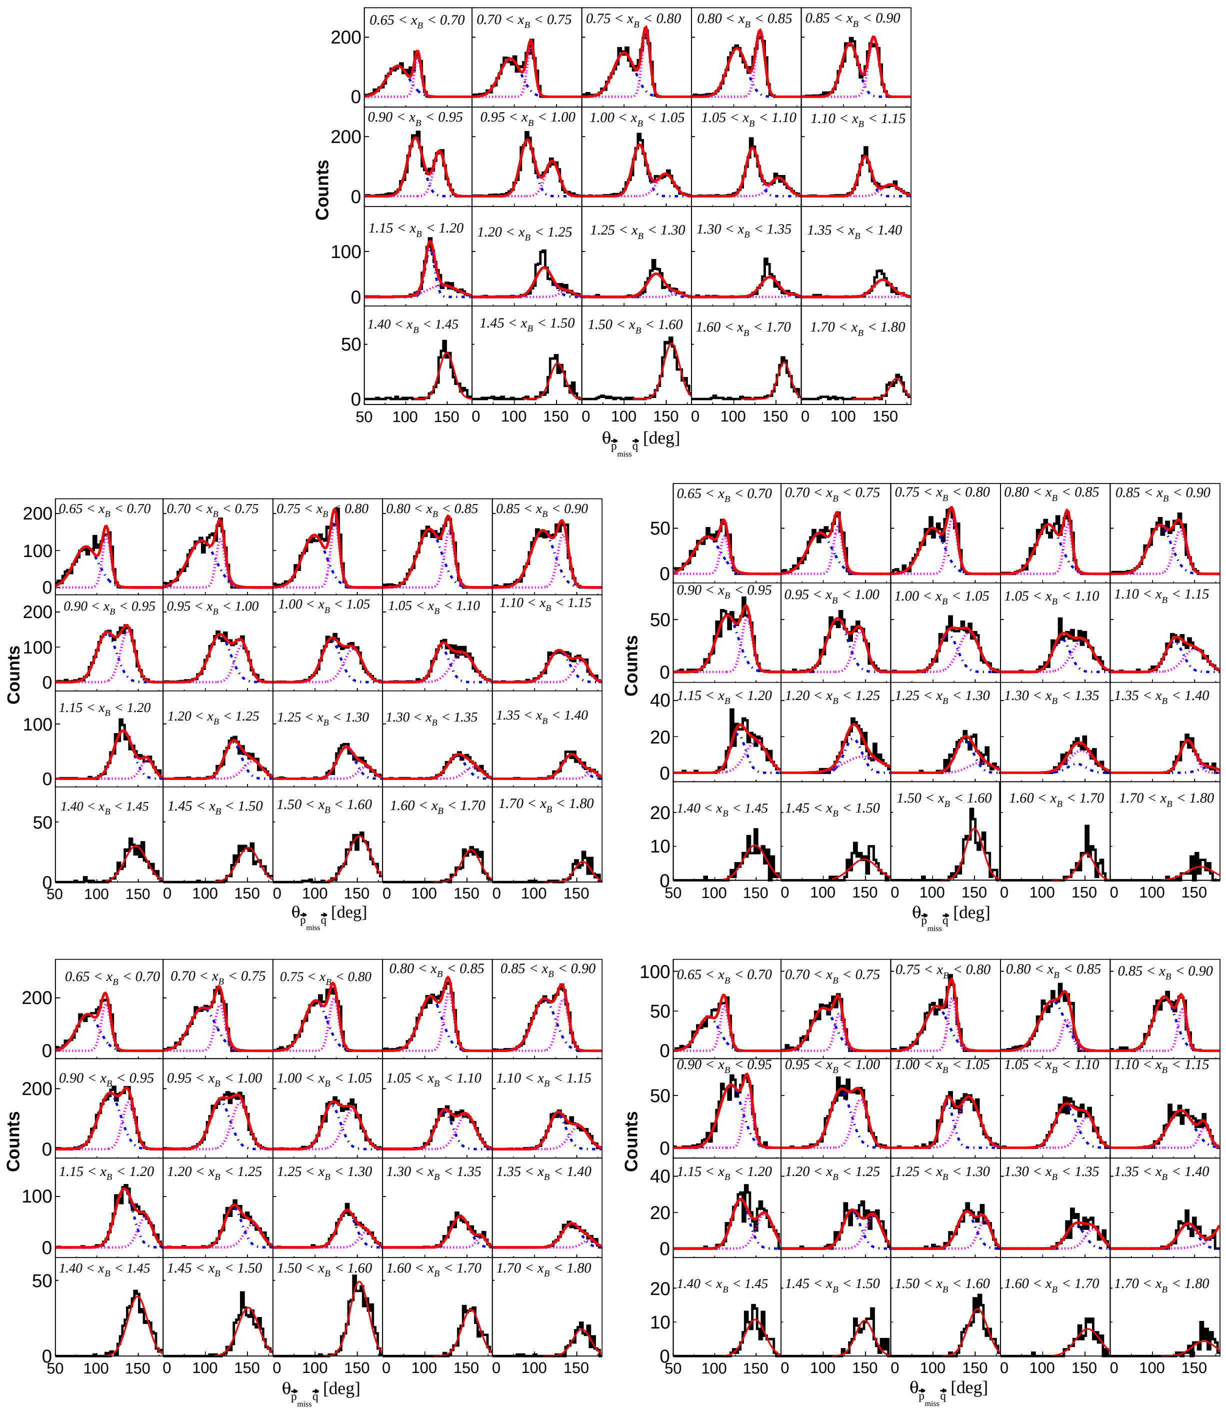


**Fig. S2: Opening angle between the missing momentum and the virtual photon.** The number of $(e, e'p)$ events plotted vs. $\theta_{\vec{p}_{miss},\vec{q}}$, the opening angle between $\vec{p}_{miss}$ and $\vec{q}$, for different bins in $x_B$ for D (top), C (middle left), Al (middle right), Fe (bottom left) and Pb (bottom right). The data were cut on $Q^2 \geq 1.5$ GeV$^2$, $\theta_{pq} \leq 25^\circ$, and $350 \leq p_{miss} \leq 600$ MeV/c. The black histogram shows all events, the blue dot-dashed curve and the magenta dotted curves show the Gaussian fits to the two peaks and the total is shown by the solid red line. The intersection of the two Gaussians is used as the angular cut for the dashed histograms in Fig. S1. At $x_B \geq 1.4$ only one Gaussian is fit to the data because the inelastic contribution is negligible.

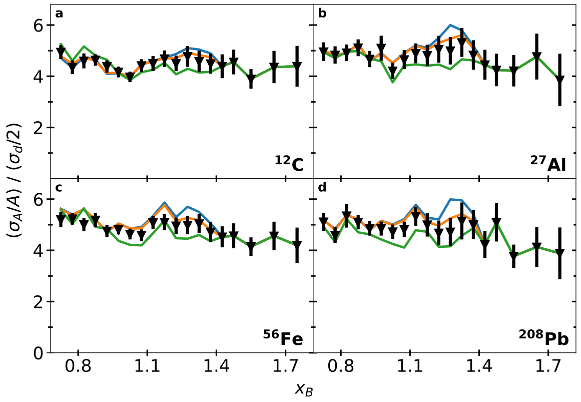


**Fig. S3: Angle cut sensitivity.** Measured per-nucleon cross section ratios for carbon to deuterium with different cuts on $\theta_{\vec{p}_{miss},\vec{q}}$. The black points correspond to the nominal cut values, the green and orange lines show the effect of increasing or decreasing the cut by 5°, respectively, and the blue line shows the effect of not applying any $\theta_{\vec{p}_{miss},\vec{q}}$ cut.

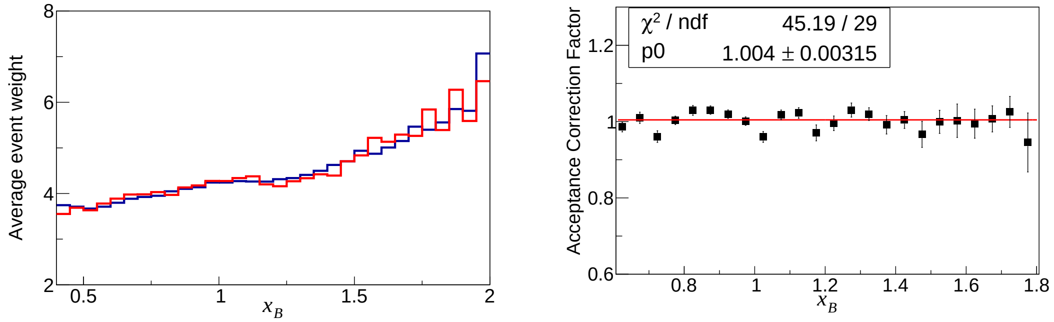


**Fig. S4: Acceptance correction.** (left) The average acceptance weight for $(e, e'p)$ events from the solid (blue histogram) and deuterium (red histogram) targets as a function of $x_B$ and (right) the acceptance correction factors for the cross section ratios, i.e., the ratio of deuterium- to solid-target acceptance-correction weights, as a function of $x_B$. The points show the data and the error bars show the $1\sigma$ or 68% confidence limits. The red line shows a constant fit to the data.

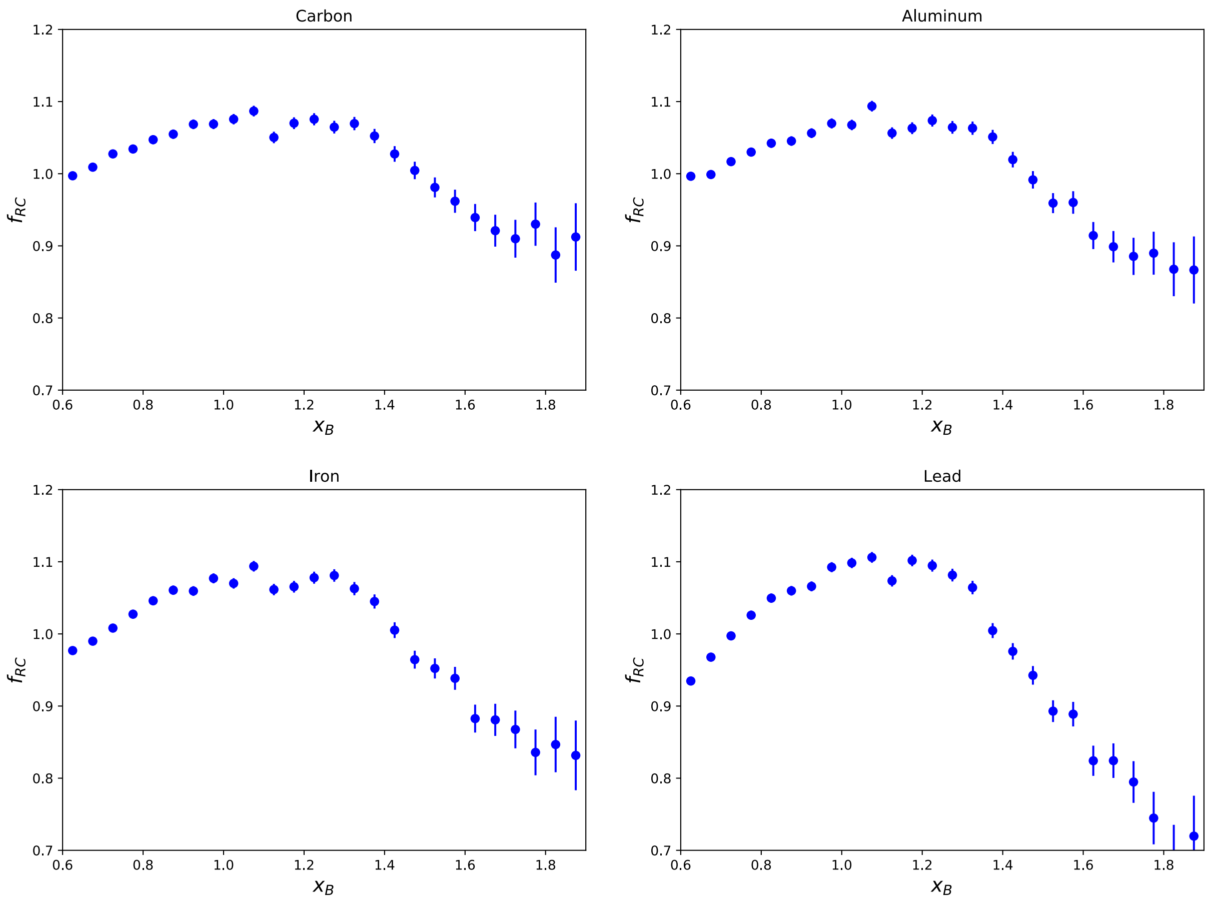


**Fig. S5: Radiative and coulomb corrections.** The combined radiative and Coulomb corrections, $RC_{A/d}(x_B)$, for $(e,e'p)$ events for nucleus $A$ relative to the deuteron for (a) carbon, (b) aluminum, (c) iron, and (d) lead. The points show the correction factors and the error bars show the $1\sigma$ or 68% confidence limits.

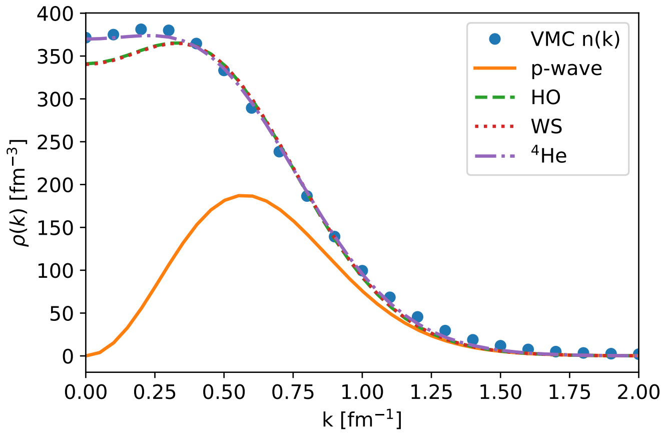


**Fig. S6: Calculated nucleon momentum distributions in $^{12}$C.** The filled blue circles represent the total momentum distribution $n(k)$ of $^{12}$C computed within the QMC method. The solid orange line shows the sum of the p-wave overlaps between the $^{12}$C and $^{11}$B+p QMC wave functions. The momentum distributions obtained by adding to the p-wave overlaps the different prescription for the s-wave contribution are displayed by the green dashed line (harmonic oscillator), dotted red line (Wood-Saxon) and dash-dotted purple line (s-wave overlaps between $^4$He and the $^3$H+p QMC wave functions). The high-momentum contributions of long- and short-range correlations are not visible on this linear scale.

**Table SI:** Event selection cut ranges

| Cut Type | Nominal Value | $1\sigma$ |
|---|---|---|
| $p_{miss}$ minimum [GeV/c] | 0.3 | 0.015 |
| $p_{miss}$ maximum [GeV/c] | 0.6 | 0.015 |
| $M_{miss}$ minimum [GeV/c$^2$] | 0.8 | 0.05 |
| $M_{miss}$ maximum [GeV/c$^2$] | 1.08 | 0.05 |
| $\theta_{pq}$ | 25° | 0.5° |
| $Q^2$ [(GeV/c)$^2$] | 1.5 | 0.01 |

[1] W. H. Dickhoff, C. Barbieri, *Prog. Part. Nucl. Phys.* **52**, 377 (2004).
[2] L. Frankfurt, M. Strikman, *Phys. Rep.* **160**, 235 (1988).
[3] C. Ciofi degli Atti, *Phys. Rept.* **590**, 1 (2015).
[4] R. Subedi, *et al.*, *Science* **320**, 1476 (2008).
[5] O. Hen, G. A. Miller, E. Piasetzky, L. B. Weinstein, *Rev. Mod. Phys.* **89**, 045002 (2017).
[6] K. Egiyan, *et al.*, *Phys. Rev. Lett.* **96**, 082501 (2006).
[7] S. Paschalis, M. Petri, A. O. Macchiavelli, O. Hen, E. Piasetzky, *Phys. Lett. B* **800**, 135110 (2020).
[8] R. Cruz-Torres, *et al.*, *Nature Physics* **17**, 306 (2020).
[9] L. Frankfurt, M. Strikman, D. Day, M. Sargsyan, *Phys. Rev. C* **48**, 2451 (1993).
[10] O. Hen, B.-A. Li, W.-J. Guo, L. B. Weinstein, E. Piasetzky, *Phys. Rev. C* **91**, 025803 (2015).
[11] R. Cruz-Torres, *et al.*, *Phys. Lett.* **B785**, 304 (2018).
[12] R. Weiss, R. Cruz-Torres, N. Barnea, E. Piasetzky, O. Hen, *Phys. Lett. B* **780**, 211 (2018).
[13] H. Hakobyan, *et al.*, *Nucl. Instrum. Meth.* **A592**, 218 (2008).
[14] B. A. Mecking, *et al.*, *Nucl. Instrum. Meth.* **A503**, 513 (2003).
[15] M. Duer, *et al.*, *Nature* **560**, 617 (2018).
[16] K. Egiyan, *et al.*, *Phys. Rev. C* **68**, 014313 (2003).
[17] N. Fomin, *et al.*, *Phys. Rev. Lett.* **108**, 092502 (2012).
[18] B. Schmookler, *et al.*, *Nature* **566**, 354 (2019).
[19] O. Hen, *et al.*, *Science* **346**, 614 (2014).
[20] A. Schmidt, *et al.*, *Nature* **578**, 540 (2020).
[21] R. Weiss, B. Bazak, N. Barnea, *Phys. Rev.* **C92**, 054311 (2015).
[22] J. Pybus, *et al.*, *Phys. Lett. B* **805**, 135429 (2020).
[23] M. Patsyuk, *et al.* (2021).
[24] E. Wolin, Clas - geant simulation (1996).
[25] E. J. Moniz, *et al.*, *Phys. Rev. Lett.* **26**, 445 (1971).
[26] R. Shneor, *et al.*, *Phys. Rev. Lett.* **99**, 072501 (2007).
[27] E. O. Cohen, *et al.*, *Phys. Rev. Lett.* **121**, 092501 (2018).
[28] R. Ent, *et al.*, *Phys. Rev.* **C64**, 054610 (2001).
[29] A. Aste, K. Hencken, J. Jourdan, I. Sick, D. Trautmann, *Nucl. Phys.* **A743**, 259 (2004).
[30] J. Kelly, *Adv. Nucl. Phys.* **23**, 75 (1996).
[31] R. B. Wiringa, V. G. J. Stoks, R. Schiavilla, *Phys. Rev. C* **51**, 38 (1995).
[32] https://www.phy.anl.gov/theory/research/overlaps/.
[33] J. Carlson, *et al.*, *Rev. Mod. Phys.* **87**, 1067 (2015).
[34] D. Dutta, *et al.*, *Phys. Rev. C* **68**, 064603 (2003).
[35] R. Weiss, *et al.*, *Phys. Rev. C* **103**, L031301 (2021).
